# Supplementary material for: Input Convex Neural Networks for Optimal Voltage Regulation
Source: arXiv:2002.08684 source file (2020-02-21)
Supplement: Supplementary file 1 [file appendix.tex]

\subsection{Appendix A}
\label{Appendix A}
\begin{proof}
	Lemma \ref{lem:max} follows from well established facts in function analysis stating that piecewise linear functions are dense in the space of all continuous functions over compact sets~\cite{royden2010real} and convex piecewise linear functions are dense in the space of all convex continuous functions~\cite{cox1971algorithm,gavrilovic1975optimal}. Using the fact that convex piecewise linear functions can be represented as a maximum of affine functions~\cite{magnani2009convex,wang2004general} gives the desired result in the lemma. 

	Lemma 1 shows that all continuous Lipschitz convex functions $f(\bd x): \mathbb{R}^d \rightarrow \mathbb{R}$ over convex compact sets can be approximated using maximum of affine functions. Then it suffices to show that an ICNN can exactly represent a maximum of affine functions. To do this, we first construct a neural network with ReLU activation function with both positive and negative weights that can represent a maximum of  affine functions. Then we show how to restrict all weights to be nonnegative.
	
	As a starting example, consider a maximum of two affine functions
	\begin{equation} \label{eqn:max_two}
	f_{CPL}(\bd x) = \max\{\bd a_1^T \bd x+b_1, \bd a_2^T \bd x + b_2\}.
	\end{equation}
	To obtain the exact same function using a neural network, we first rewrite it as
	\begin{equation}
	f_{CPL}(x) =  (\bd a_2^T \bd x+b_2) + \max\left((\bd a_1-\bd a_2)^T \bd x + (b_1-b_2), 0\right).
	\end{equation}
	Now define a two-layer neural network with layers $\bd z_1$ and $\bd z_2$ as shown in Fig.~\ref{fig:twolayer}:
	\begin{subequations}
		\label{two_layer_NN}
		\begin{align}
		z_1 &= \sigma \left((\bd a_1-\bd a_2)^T \bd x + (b_1-b_2)\right)\,,\\
		z_2 &= z_1+ \bd a_2^T \bd x + b_2\,
		\end{align}
	\end{subequations}
	
	where $\sigma$ is the ReLU activation function and the second layer is linear. By construction, this neural network is the same function as $f_{CPL}$ given in \eqref{eqn:max_two}.
	
	\begin{figure}[h]
		\centering
		\includegraphics[width=0.6 \columnwidth]{Figures/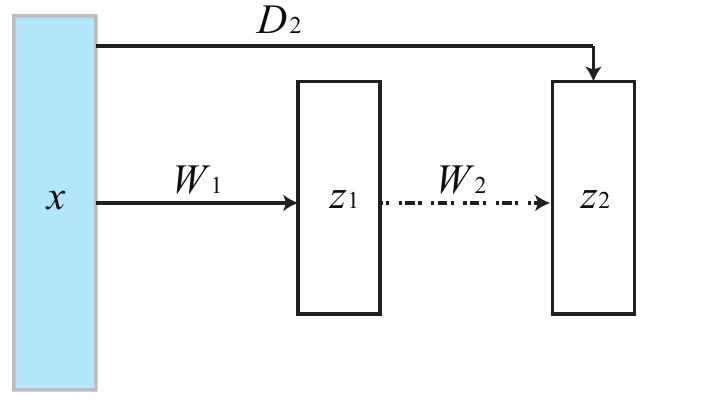}
		\caption{A simple two-layer neural networks. In alignment with \eqref{two_layer_NN}, $W_1$ denotes the first-layer weights $\bd a_1-\bd a_2$ and bias $b_1-b_2$, and $W_2$ denotes the linear second layer. Direct layer is denoted as $D_2$ for weights $\bd a_2$ and bias $b_2$.}
		\label{fig:twolayer}
	\end{figure}
	
	The above argument extends directly to a maximum of  $K$ linear functions. Suppose
	\begin{equation}
	f_{CPL}(\bd x)= \max\{\bd a_1^T \bd x + b_1, ..., \bd a_K^T \bd x+b_K\}
	\end{equation}
	Again the trick is to rewrite $f_{CPL}(\bd x)$ as a nested maximum of affine functions. For notational convenience,  let $L_i = \bd a_i^T \bd x+b_i$, $L'_i = L_i-L_{i+1}$. Then
	\begin{align*}
	f_{CPL} &= \max\{L_1, L_2, ..., L_K\}\, \nonumber\\
	& = \max\{\max\{L_1, L_2, ..., L_{K-1}\}, L_K\}\,\nonumber\\
	& = L_K + \sigma \left(\max\{L_1, L_2, ..., L_{K-1}\}-L_K\right) \nonumber\\
	& = L_K + \sigma\left(\max\{\max\{L_1, L_2, ..., L_{K-2}\}, L_{K-1}\}-L_K,0\right)\,\nonumber\\
	& = L_K + \sigma\left(L_{K-1}-L_K+\sigma\left(\max\{L_1, L_2, ..., L_{K-2}\}-L_{K-1}, 0\right),0\right) \nonumber\\
	% & = L_K + \max\{L'_{K-1}+\max\{L'_{K-2}+\max\{\max\{L_1, L_2, ..., L_{K-3}\}-L_{K-2}, 0\}, 0\},0\}\, \nonumber\\
	&= ... \nonumber\\
	& = L_K + \sigma\left(L'_{K-1}+\sigma\left(L'_{K-2}+\sigma\left(...\sigma\left(L'_2+\sigma\left(L_1-L_2, 0\right), 0\right), ..., 0\right), 0\right),0\right).
	\end{align*}
	The last equation describes a $K$ layer neural network, where the layers are:
	\begin{align*}
	z_1 &= \sigma\left(L_1-L_2, 0\right) =  \sigma\left((\bd a_1-\bd a_2)^T \bd x + (b_1-b_2)\right)\,,\\
	z_2 & =  \sigma\left(L_2'+ z_1, 0\right) =  \sigma \left(z_1+ (\bd a_2-\bd a_3)^T \bd x+(b_2-b_3)\right)\,,\\
	... &... \\
	z_{i} &= \sigma\left(L'_i+z_{i-1}, 0\right) = \sigma \left(z_{i-1}+ (\bd a_i- \bd a_{i+1})^T \bd x+(b_{i}-b_{i+1})\right)\,,\\
	... &... \\
	z_{K} &= z_{K-1} + L_K = h_{K}\left(z_{K-1}+ L_{K}\right) = \left(z_{K-1}+ \bd a_K^T \bd x+b_K \right).
	\end{align*}
	Each layer of of this neural network uses only a single activation function.
	
	Although the above neural network exactly represent a maximum of  linear functions, it is not convex since the coefficients between layers could be negative. In particular, each layer involves an inner product of the form $(\bd a_i- \bd a_{i+1})^T \bd x$ and the coefficients are not necessarily nonnegative. To overcome this, we simply expand the input to include $\bd x$ and $-\bd x$. Namely, define a new input $\hat{\bd x} \in \R^{2d}$ as
	\begin{equation}\label{eqn:hatx}
	\hat{\bd x} = \begin{bmatrix} \bd x \\ -\bd x\end{bmatrix}.
	\end{equation}
	Then any inner product of the form $\bd h^T \bd x$ can be written as
	\begin{align*}
	\bd h^T \bd x & = \sum_{j=1}^d h_i x_i \\
	& = \sum_{i:h_i \geq 0} h_i x_i + \sum_{i:h_i < 0} h_i x_i \\
	& = \sum_{i:h_i \geq 0} h_i x_i+ \sum_{i:h_i <0 } (-h_i)(-x_i) \\
	& = \sum_{i:h_i \geq 0} h_i \hat{x}_i+ \sum_{i:h_i <0 } (-h_i)(\hat{x}_{i+d}),
	\end{align*}
	where all coefficients are nonnegative in the above sum.
	
	Therefore any inner product between a coefficient vector and the input $\bd x$ can be written as an inner product between a nonnegative coefficient vector and the expanded input $\hat{\bd x}$. Therefore, without loss of generality, we can limit all of the weights between layers to be nonnegative, and thus the neural network to be input convex. Note that in optimization problems, we need to enforce consistency in $\hat{\bd x}$ be including \eqref{eqn:hatx} as a constraint. However, this is a linear equality constraint, which maintains the convexity of the optimization problem.
	
\end{proof}

\subsection{Appendix B}
\label{Appendix B}
\begin{proof}
	The second statement of Theorem \ref{thm:complexity} directly follows the construction in the proof of Theorem \ref{thm:power}, which shows that a maximum of $K$ affine functions can be represent by a $K$-layer ICNN (with a single ReLU function in each layer). So it remains to show the first statement of Theorem \ref{thm:complexity}.
	
	To show that a maximum of affine functions can require exponential number of pieces to approximate a function specified by an ICNN with $K$ activation functions, consider a network with 1 hidden layer of K nodes and the weights of direct ``passthrough'' layers are set to 0:
	\begin{equation}
	f_{ICNN}(\bd x) = \sum_{i=1}^{K} w_{1i} \sigma(\bd w_{0i}^T \bd x + b_i)\,,
	\end{equation}
	It contains $3K$ parameters: $\bd w_{0i}$, $w_{1i}$ and $b_i$, where $\bd w_{0i} \in \R^{d}$ and $w_{1i}, b_i \in \R$.
	
	In order to represent the same function by a maximum of affine functions,  we need to assess the value of every activation unit $\sigma(\bd w_{0i}^{T} \bd x + b_i)$. If $\bd w_{0i}^{T} \bd x + b_i \geq 0$, $\sigma(\bd w_{0i}^{T} \bd x + b_i) = \bd w_{0i}^{T} \bd x + b_i$; otherwise, $\sigma(\bd w_{0i}^{T} \bd x + b_i) = 0$. In total, we have $2^K$ potential combinations of piecewise-linear function, including
	\begin{align*}
	L_1\ \ = & \left(\sum_{i=1}^{K} w_{1i} \bd w_{0i}\right)^T \bd x + \sum_{i=1}^{K} w_{1i} b_i\,, \text{if all\ \ } \bd w_{0i}^{T} \bd x + b_i \geq 0\\
	L_2\ \ =& \left(\sum_{i=2}^{K} w_{1i} \bd w_{0i}\right)^T \bd x + \sum_{i=2}^{K} w_{1i} b_i\,, \\
	& \text{if\ } \bd w_{01}^T \bd x + b_1 < 0 \text{ and all other } \bd w_{0i}^{T} \bd x + b_i \geq 0\\
	L_3\ \ =& \left(w_{11} \bd w_{01}  + \sum_{i=3}^{K} w_{1i} \bd w_{0i}\right)^T \bd x + w_{1i} b_i + \sum_{i=3}^{K} w_{1i} b_i\,,\\
	& \text{if\ } \bd w_{02}^{T} \bd x + b_2 < 0 \text{\ and other } \bd w_{0i}^{T} \bd x + b_i \geq 0\\
	& \ \ \ \ \cdots \cdots\,,\\
	L_{2^K} =&0\,, \text{  if all }\bd w_{0i}^{T} \bd x + b_i < 0.
	\end{align*}
	So the following maximum over $2^K$ pieces is required to represent the single linear ICNN:
	$$\max\{L_1, L_2, ..., L_{2^K}\}. $$
\end{proof}
